# Supplementary material for: Noncollinear magnetic sampling method for paramagnetic Mott insulator MnO
Source: arXiv:1810.05416 source file (2019-05-20)
Supplement: Supplementary file 1 [file PCCP-SI.pdf]

**Supporting Information for**

# A "non-dynamical" way of describing room-temperature paramagnetic manganese oxide

Sangmoon Yoon,[1,2] Seoung-Hun Kang,[2,a)] Sangmin Lee,[1,2] Kuntae Kim,[1] Jeong-Pil Song,[2,b)] Miyoung Kim,[1,c)] and Young-Kyun Kwon[2,d)]

[1)] *Department of Materials Science and Engineering, Seoul National University, Seoul, 08826, Korea*

[2)] *Department of Physics and Research Institute for Basic Sciences, Kyung Hee University, Seoul, 02447, Korea*

---

[a)] Present address: Korea Institute for Advanced Study (KIAS), Seoul, 02455, Korea

[b)] Present address: Department of Chemistry, Brown University, Providence, RI, 02912, USA

[c)] Corresponding author. E-mail: mkim@snu.ac.kr

[d)] Corresponding author. E-mail: ykkwon@khu.ac.kr

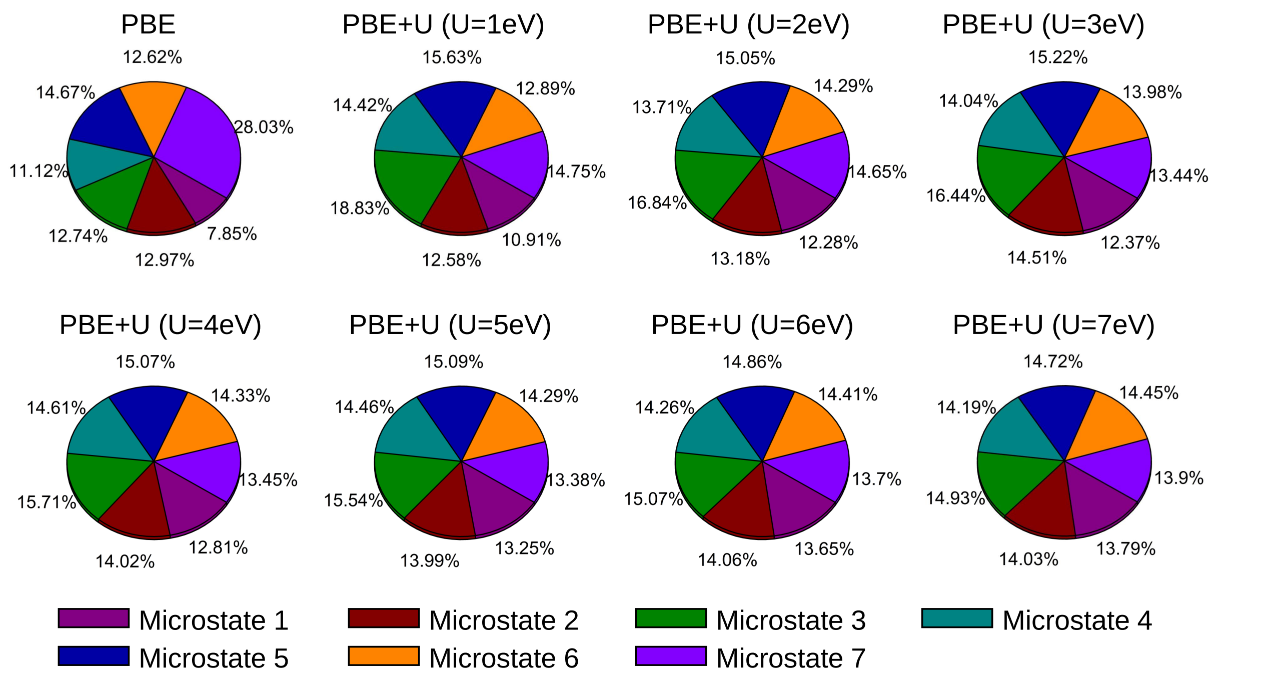


FIG. S1. (Color online) Probability of finding the specific microstate among the seven different disordered states at $T = 300$ K. The probability is estimated with various values of on-site Coulomb interaction $U$. For a given $u$ value, the corresponding probability distribution was used to calculate various room-temparture properties of paramagnetic MnO, whereas for the estimation of Néel temperature, the probability distribution was reevaluated at each temperature. Based on the distribution of $U = 4$ eV, the probability of finding each microstructure is in the range of 12 to 16 %, which indicates that no particular microstates are dominant in the ensemble of paramagnetic MnO.

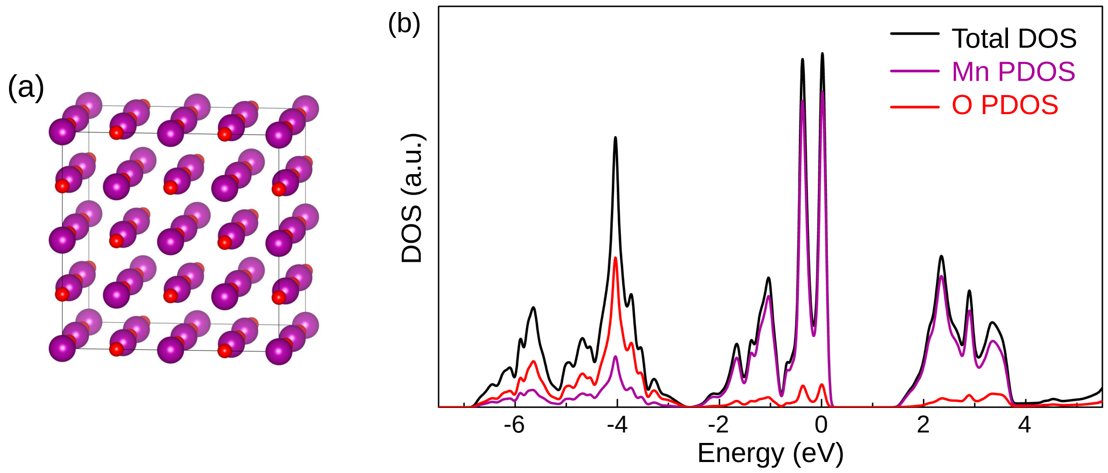


FIG. S2. (a) Schematic illustration of nonmagnetic MnO phase, where Mn ions ions do not have local magnetic moments. (b) DOS of nonmagnetic MnO phase calculated with $U$ = 4 eV. The black solid line represents the total DOS; the purple and red solid lines indicate the partial DOSs of Mn and O, respectively. The localized state at the Fermi level is formed due to the strong on-site Coulomb interaction, but it is still metallic in the nonmagnetic phase.

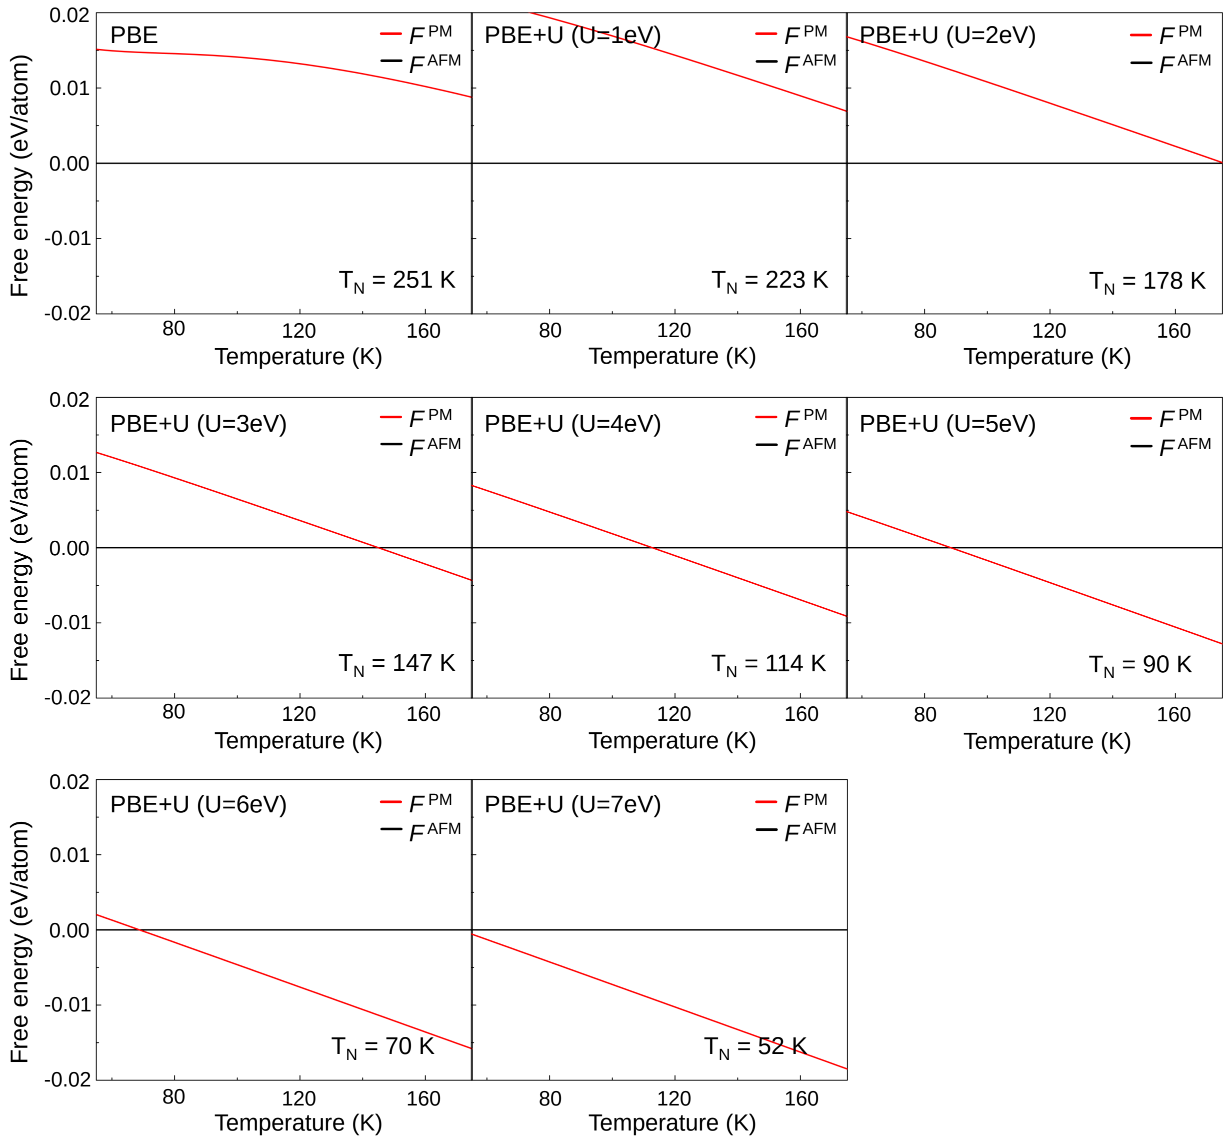


FIG. S3. (Color online) Per-atom Helmholtz free energy of paramagnetic (PM, red solid line) MnO relative to that of antiferromagnetic (AFM, black solid line) MnO, which is set to zero, obtained with various values of on-site Coulomb interaction $U$. The crossover temperature corresponding to Néel temperature decrease 250K to 50K with increasing $U$.

## Algorithm to generate a disordered magnetic structure for NCMSM

The goal of the algorithm is to generate a noncollinearly disordered magnetic structure which satisfies the following three conditions: (i) local magnetic moments are oriented in randomly different directions in three dimensions; (ii) the magnitude of each local magnetic moment is 4.58 $\mu_B$; and (iii) the total magnetic moment or the vector sum of all local magnetic moments in the supercell, is zero. To generate such a magnetic structure, we proceeded with the following procedure. We constructed a $2 \times 2 \times 2$ supercell consisting of 32 manganese and 32 oxygen atoms. To assign the magnetic moments localized at the thirty two manganese atoms, we used two random number generators to determine respectively the polar and azimuthal angles of each of the first 30 local magnetic moments. Then, we adjusted the orientation of the remaining two unassigned local magnetic moments to make the total magnetic moment to be zero. As a last step, we randomly mixed the order of the local magnetic moments.

## Details of individual self-consistent field (SCF) calculations

It should be noted that the PBE+$U$ calculations were carried out without constraining the magnetic moments. Figure S4 shows the direction and magnitude of magnetic moments before and after the SCF calculations. This result was obtained with $U = 4$ eV in one of the magnetic samples we used. Despite of the non-constrained calculations, the final directions of the magnetic moments (after SCF) did not change significantly compared with their initial directions. This implies that the energy surface of magnetically disordered MnO is quite bumpy and has a number of local minima. In this case, the total magnetic moment was computed to be 0.99 $\mu_{\mathbf{B}}$, which is quite small in comparison with the local magnetic moment value, 4.58 $\mu_{\mathbf{B}}$, of each manganese ion. Over all the magnetic samples, the total magnetic moments were distributed between 0.31 $\mu_{\mathbf{B}}$ and 1.42 $\mu_{\mathbf{B}}$.

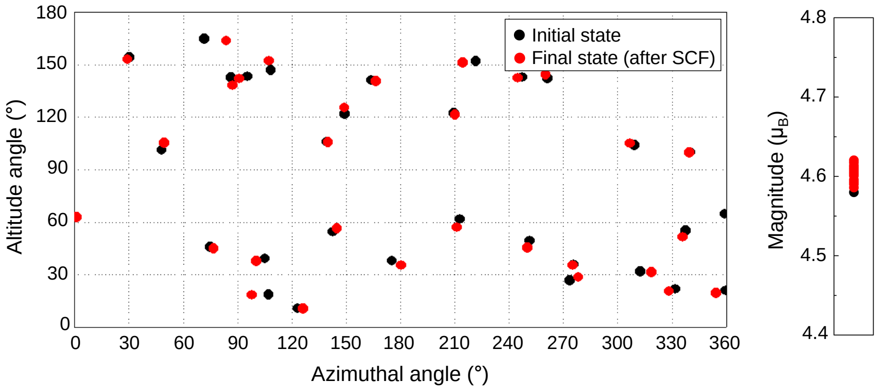


FIG. S4. Initial magnetic moments created by the way described in **Algorithm to generate a disordered mangnetic structure for NCMSM**, and final magnetic moments obtained after the SCF calculation. The black and red dots denote the magnetic moments before and after the SCF calculation, respectively. The left and right graphs show the orientations and magnitudes of all local magnetic moments, respectively. This result was obtained with $U = 4$ eV in one of the magnetic samples we used.

## Deviations caused by the limited number of magnetic samples

In principle, should there be more magnetic samples, we would describe the paramagnetic properties better. The seven different disordered structures are used in this study. To check the sampling size dependence, we carried out our calculations for four newly generated magnetic samples only with $U = 4$ eV. Figure  shows the calculated free energies of eleven different samples with randomly noncollinearly disordered magnetic structures and their accumulated ensemble averaged free energy. After seventh iteration, the accumulated ensemble averaged energy is within $\pm 0.001$ eV/unit from the reference energy, which is the ensemble averaged value after eleventh iteration, as shown in Fig. . Apparently, a higher accuracy will be achieved if more magnetic samples are used.

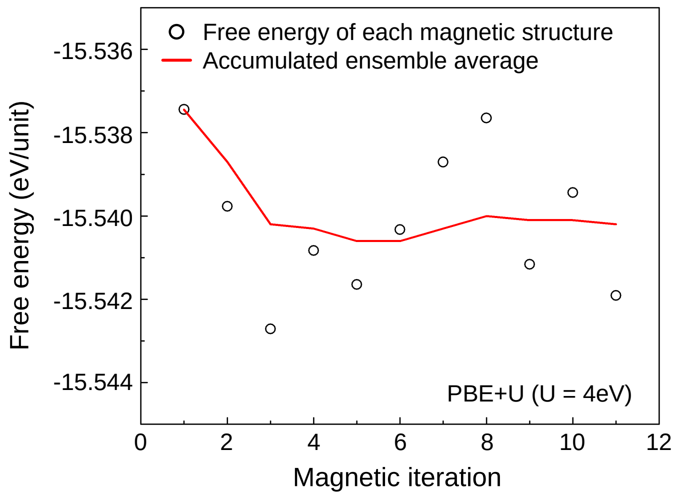


FIG. S5. (Color online) The calculated free energy of individual magnetic configurations and the accumulated ensemble averaged free energy. The black circles indicate the free energies of individual magnetic samples and the red line denotes the accumulated ensemble averaged energy.

## Distribution of local magnetic moments in MSM+$U$

To check whether MSM+$U$ yields similar values of local magnetic moments to those obtained by NCMSM+$U$, we carried out MSM+$U$ calculation. Figure **??** shows the distribution of local magnetic moments estimated with $U_{\text{eff}} = 4$ eV by MSM+$U$ as well as those evaluated with various $U$ values by NCMSM+$U$. The MSM+$U$ calculation with $U_{\text{eff}} = 4$ eV yields the distribution which is in good agreement with the experiments. The magnitudes of the local magnetic moments evaluated using MSM+$U$ with $U_{\text{eff}} = 4$ eV are distributed around their average value of 4.60 $\mu_B$, which is essentially the same as the mean value of 4.59 $\mu_B$ calculated by NCMSM+$U$, although the specific shape of distribution is a little bit different. This indicates that although the collinear calculation yields similar values of the local magnetic moments as the noncollinear one does, the spin noncollinearity plays an important role in the electronic structures and the phase transition behaviors of paramagnetic manganese oxides.

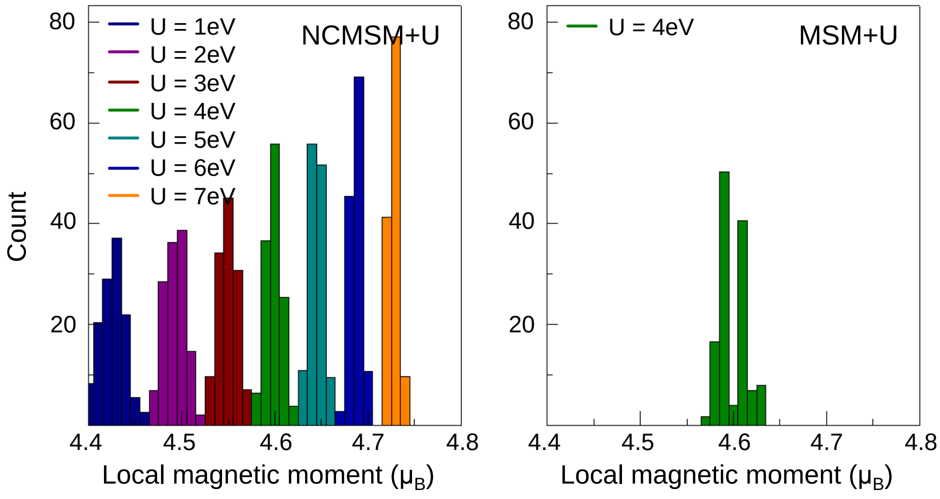


FIG. S6. (Color online) The distribution of local magnetic moments of paramagnetic MnO. The left and right sides are the distribution estimated by NCMSM+$U$ and MSM+$U$, respectively. The distributions for different $U$ values are represented by different color. The distribution for the $U_{\text{eff}}$ (or $U$) = 4 eV case is represented by the olive-colored sticks
